# Supplementary material for: PromptRobust: Towards Evaluating the Robustness of Large Language Models on Adversarial Prompts
Source: arXiv:2306.04528 source file (2024-07-16)
Supplement: Supplementary file 1 [file tb-appendix-new-datasets.tex]

\begin{table}[!ht]
\caption{Attack results of T5, UL2, Llama2 and Vicuna-v1.3 on new datasets.}

\label{tb-append-new-dataset-model}
    \centering
    \resizebox{0.48\textwidth}{!}{
    \begin{tabular}{ccccc}
    \toprule
        ~ & T5 & UL2 & Llama2 & Vicuna-v1.3 \\ \midrule
        Valid Parentheses & 0.71\scriptsize{$\pm$0.34} & 0.15\scriptsize{$\pm$0.06} & 0.64\scriptsize{$\pm$0.62} & 0.11\scriptsize{$\pm$1.41} \\
        Bool Logic & 0.20\scriptsize{$\pm$0.21} & 0.11\scriptsize{$\pm$0.03} & 0.76\scriptsize{$\pm$0.27} & -0.31\scriptsize{$\pm$1.98} \\ \bottomrule
    \end{tabular}
    }
\end{table}

\begin{table}[!ht]
\caption{Attack results of different attacks on new datasets.}
\label{tb-append-new-dataset-attack}
    \centering
    \resizebox{.48\textwidth}{!}{
    \begin{tabular}{ccccccc}
    \toprule
        ~ & BertAttack & TextBugger & DeepWordBug & TextFooler & CheckList & StressTest \\ \midrule
        Valid Parentheses & 0.70\scriptsize{$\pm$0.40} & 0.79\scriptsize{$\pm$0.34} & 0.77\scriptsize{$\pm$0.37} & 0.81\scriptsize{$\pm$0.35} & 0.61\scriptsize{$\pm$0.37} & -0.29\scriptsize{$\pm$1.10} \\
        Bool Logic & 0.89\scriptsize{$\pm$0.23} & 0.67\scriptsize{$\pm$0.37} & 0.50\scriptsize{$\pm$0.43} & 0.84\scriptsize{$\pm$0.33} & 0.17\scriptsize{$\pm$0.58} & -0.59\scriptsize{$\pm$2.02} \\ \bottomrule
    \end{tabular}
    }
\end{table}
