# Supplementary material for: PromptRobust: Towards Evaluating the Robustness of Large Language Models on Adversarial Prompts
Source: arXiv:2306.04528 source file (2024-07-16)
Supplement: Supplementary file 2 [file tb-appendix-new-llms.tex]

\begin{table*}[!ht]
\caption{Attack results of Vicuna-13B-v1.3 and Llama2-13B-chat.}
\label{tb-appendix-new-llms}
    \centering
    \resizebox{.8\textwidth}{!}{
    \begin{tabular}{l c c c c c c c c c c}
    \toprule
        Model & SST-2 & CoLA & QQP & MRPC & MNLI & QNLI & RTE & WNLI & MMLU & Math \\ \midrule
        Vicuna-v1.3 & 0.77\scriptsize{$\pm$0.26} & 0.66\scriptsize{$\pm$0.27} & 0.65\scriptsize{$\pm$0.35} & 0.51\scriptsize{$\pm$0.42} & 0.59\scriptsize{$\pm$0.36} & 0.84\scriptsize{$\pm$0.20} & 0.76\scriptsize{$\pm$0.32} & 0.68\scriptsize{$\pm$0.39} & 0.41\scriptsize{$\pm$0.44} & - \\ 
        Llama2 & 0.24\scriptsize{$\pm$0.33} & 0.38\scriptsize{$\pm$0.32} & 0.59\scriptsize{$\pm$0.33} & 0.84\scriptsize{$\pm$0.27} & 0.32\scriptsize{$\pm$0.32} & 0.51\scriptsize{$\pm$0.39} & 0.68\scriptsize{$\pm$0.39} & 0.73\scriptsize{$\pm$0.37} & 0.28\scriptsize{$\pm$0.24} & - \\ 
        GPT4* & 0.05\scriptsize{$\pm$0.02} & 0.07\scriptsize{$\pm$0.02} & - & - & - & 1\scriptsize{$\pm$0.00} & - & - & 0.04\scriptsize{$\pm$0.00} & 0.63\scriptsize{$\pm$0.24} \\ \bottomrule
    \end{tabular}
    }
\end{table*}
